# Supplementary material for: Norm-Range Partition: A Universal Catalyst for LSH based Maximum Inner Product Search (MIPS)
Source: arXiv:1810.09104 source file (2018-11-05)
Supplement: Supplementary file 1 [file experiment-appendix.tex]

\documentclass[a4paper]{article}
\usepackage[top=1in, bottom=1in, left=1.25in, right=1.25in]{geometry}
\usepackage{pgfplots}
\usepackage{pgfplotstable}
\usepackage{blindtext}
\usepackage{graphicx}
\usepackage{subcaption}
\usepgfplotslibrary{units}
\pgfplotsset{width=7cm,compat=1.13}
\pgfplotsset{major grid style={dotted,gray!50!black}}
\newcommand{\figurewidth}{0.8}
\newcommand{\figuregap}{-2.8em}
\newcommand{\figurepercentperrow}{0.288}
\pgfplotsset{every axis/.append style={
		label style={font=\tiny},
		tick label style={font=\tiny}  
}}
\begin{document}
\input{append-top1}
\input{append-top10}
\input{append-top50}
\input{append-bit16}
\input{append-bit64}
\end{document}
